# Supplementary material for: Solution for CVPR 2024 UG2+ Challenge Track on All Weather Semantic Segmentation
Source: arXiv:2406.05837 source file (2024-06-09)
Supplement: Supplementary file 1 [file X_suppl.tex]

\section{Conclusion}

In this report, we introduce an InternImage-based approach for semantic segmentation under adverse weather conditions. To mitigate the limitations of existing datasets and the challenges presented by such conditions, we employ both offline and online data augmentation techniques to enhance the training set. Our method leverages InternImage as the semantic segmenter, with UperNet serving as the backbone network. Experimental results demonstrate that our proposed solution achieves exceptional performance on the test set in the UG2+ Challenge 2024.
